# Supplementary material for: Optimal Trajectories of a UAV Base Station Using Hamilton-Jacobi Equations
Source: arXiv:2102.02632 source file (2021-02-04)
Supplement: Supplementary file 1 [file appendix-H.tex]

% appendix-H.tex%
\subsection{Proof of formula \eqref{dp/dt:eq}
% with Hamilton equations}
using Hamilton equations of movement
\label{app:concatenated}}
\noindent
Hamilton equations result 
from the  Legendre Transform differential 
properties 
and from
the Lagrange movement equations
(a single-phase is considered here):
%%%
\begin{subequations}
%%%%
\begin{eqnarray}
\ddtime {p} &=& - \dpart{H}{x}
\label{Hamilton-a:eq}
\\[1mm]
\ddtime {x} &=& \dpart{H}{p}
\label{Hamilton-b:eq}
\end{eqnarray}
%%%
\end{subequations}
Thus for the quadratic repulsive model adopted here:
%%%
\begin{subequations}
\begin{eqnarray}
\ddtime{p} &=& \w^2\ x	% -> corrected
\label{Hamilton-a-repulsive:eq}
\\[1mm]
\ddtime x &=& p
\label{Hamilton-b-repulsive:eq}
\end{eqnarray}
\end{subequations}
%%%
Define
the %{\em concatenated} 
state vector 
as
$Y = \trivec{p}{\w\ x} 
\in E_c = \bR^n \oplus \bR^n$
.
Previous differential system writes then:
\begin{eqnarray}
\ddtime Y &= \w\ A\ Y &
\end{eqnarray}
where the linear "{\bf exchange}" operator 
$A$ of $E_c$ is defined as: %defined by
$
A\ \trivec{u}{v} = \trivec {v}{u}
\enspace
\forall\ u,\ v \in \Real^n%E
\enspace.
$
\\
Thus for any $\tone,\ \ttwo \in {\cal I}$
\begin{equation}
Y(\ttwo)
=
\trivec{\ptwo}{\w\ \xtwo}
=
\exp\ (A\ \phase)
\
\trivec{\pone}{\w\ \xone}
\label{exp:eq}
\end{equation}
here $\phase = \w\ (\ttwo - \tone)$ 
is  the temporal {\bf phase}
as defined by \eqref{temporal-phase:eq}
\enspace.
\\
It is practical in the sequel 
to differentiate \wrt $\phase$,
by noticing that
\begin{align*}
\dpart{}{\tone} = - \w\ \dpart{}{\phase}
&&
\dpart{}{\ttwo} = +\w\ \dpart{}{\phase}
\\
\ddpart{}{\tone} =\ddpart{}{\ttwo} 
&&
= \w^2\ \ddpart{}{\phase}
\end{align*}
%\\
Now differentiating $Y(\ttwo)$
\wrt $\phase$ 
at {\bf fixed} $\xone,\ \xtwo$
yields \enspace:
%%%%
\begin{align*}
%\lefteqn{
\del Y(\ttwo) =  \trivec{\del \ptwo}{0}
%}
%\\
&=
A\ \del \phase\ 
\underbrace{
\exp\  A\ \phase \trivec{\pone}{\w\ \xone}
}_{}
%\trivec{\ptwo}{\w \xtwo}
&
+\
 \exp  A\  \phase\  \trivec{\del \pone}{0}
\nonumber
\\%[1mm]
&= 
A\ \del \phase\ \trivec{\ptwo}{\w\ \xtwo} 
&
+ \ 
\exp  A\  \phase \  \trivec{\del \pone}{0}
%%%
\end{align*}
The second component of $\del Y(\ttwo)$ 
develops thus as:
\[
0  = \del \phase\ \ptwo + \sinh \phase\ \del \pone
\label{useful-dpdphi:eq}
\qed
\]
%%%
Remark:  similarly for the variation of $\ptwo$ namely 
$\del  \ptwo$ \enspace,
we notice 
by applying inverse return - phase inversion, that 
\[
Y(\tone)
=
\trivec{\pone}{\w\ \xone}
=
\exp\ -(A\ \phase)
\
\trivec{\ptwo}{\w\ \xtwo}
\]
Reasoning as before, one finds:
\begin{align*}
\del Y(\tone) 
&=  \trivec{\del \pone}{0}
= 
- A\ \del \phase\ \trivec{\pone}{\w\ \xone} 
+ \ 
\exp  - A\  \phase \  \trivec{\del \pone}{0}
\\%[1mm]
 0 &= -\ \del \phase\ \pone - \sinh \phase\ \del \ptwo
 \qed
\nonumber
%%%
\end{align*}
Thus impulsions $\pone$ and $\ptwo$ enjoy completely similar, symmetric variations 
\wrt temporal phase $\phase$
\enspace.
\input
